# Supplementary material for: Deformable Shape Completion with Graph Convolutional Autoencoders
Source: arXiv:1712.00268 source file (2018-04-03)
Supplement: Supplementary file 1 [file appendix.tex]

\appendix
\section{Appendix}
\subsection{Network (hyper) parameters}
In Section 4 we presented the parameter values for the network implementation used in our experiments ($M=8$, $\lambda=10^{-8}$, and latent dimensionality $128$). In Tables~\ref{tab_weight_matrices}, \ref{tab_latent_dim}, and \ref{tab_latent_loss_weight} we show the effects of varying some of these values. We do not see a benefit beyond 8 weight matrices, and we do not consider a latent dimensionality beyond $128$ to avoid introducing additional model complexity.
%------ Weight Matrices ------
\begin{table}[htb]
\centering
\small
\begin{tabular}{ l@{\hskip 0.01\textwidth}c@{\hskip 0.01\textwidth}c@{\hskip 0.01\textwidth}c@{\hskip 0.01\textwidth}c@{\hskip 0.01\textwidth}c@{\hskip 0.01\textwidth}c@{\hskip 0.01\textwidth}c  }
    \hline\hline
    $M$ & $4$ 	& $8$ & $16$ \\ \hline    
      	& $0.054$ & $0.049$ & $0.050$ & \\ \hline
  \end{tabular}   
  \vspace{2mm}
\caption{\small Mean test error for varying weight matrices $M$ with fixed $\lambda=10^{-6}$ and latent dim 64.}
\label{tab_weight_matrices}	
\end{table}
%------ Latent space dimensionality ------
\begin{table}[htb]
\centering
\small
\begin{tabular}{ l@{\hskip 0.01\textwidth}c@{\hskip 0.01\textwidth}c@{\hskip 0.01\textwidth}c@{\hskip 0.01\textwidth}c@{\hskip 0.01\textwidth}c@{\hskip 0.01\textwidth}c  }
    \hline\hline
    latent dimensionality & $32$ & $64$ & $128$  \\ \hline    
      	& 0.051 & 0.049 & 0.043 \\ \hline   
  \end{tabular}   
  \vspace{2mm}
\caption{\small Mean test error for varying latent space dimensionality with fixed $M=8$ and $\lambda=10^{-6}$}
\label{tab_latent_dim}	
\end{table}
%------ Latent loss weight ------
\begin{table}[htb]
\centering
\small
\begin{tabular}{ l@{\hskip 0.01\textwidth}c@{\hskip 0.01\textwidth}c@{\hskip 0.01\textwidth}c@{\hskip 0.01\textwidth}c@{\hskip 0.01\textwidth}c@{\hskip 0.01\textwidth}c@{\hskip 0.01\textwidth}c  }
    \hline\hline
    $\lambda$ & $10^{-4}$ 	& $10^{-6}$ & $10^{-8}$ \\ \hline    
      	   & $0.053$ & $0.049$ & $ 0.041$ & \\ \hline
  \end{tabular}   
  \vspace{2mm}
\caption{\small Mean test error for varying the prior weight $\lambda$ with fixed $M=8$ and latent space dimension $64$.}
\label{tab_latent_loss_weight}	
\end{table}

\subsection{Dataset details}
As mentioned in Section 4, we train our models using human shapes from the DFAUST dataset~\cite{dfaust:CVPR:2017}. We subsample each shape consistently by a factor of 2, resulting in $3446$-vertex triangulated meshes. An example is shown in Figure~\ref{fig:receptive_field} (right). An interesting property of these sub-sampled meshes is that the spatial distribution of vertices over the shape surface is not quite uniform. We illustrate this by showing the receptive field (at the n-1 layer before embedding) for a few different vertices (see Figure~\ref{fig:receptive_field} left). As can be seen in the figure the support varies across the surface. We will provide the vertex map from the subsampled mesh to the original data, as well as all train and test splits used in our experiments.

\begin{figure}[h]
\centering
\begin{tabular}{cc}
\includegraphics[height=0.4\textwidth]{./figures/receptive_field.png} &
\includegraphics[width=0.23\textwidth]{./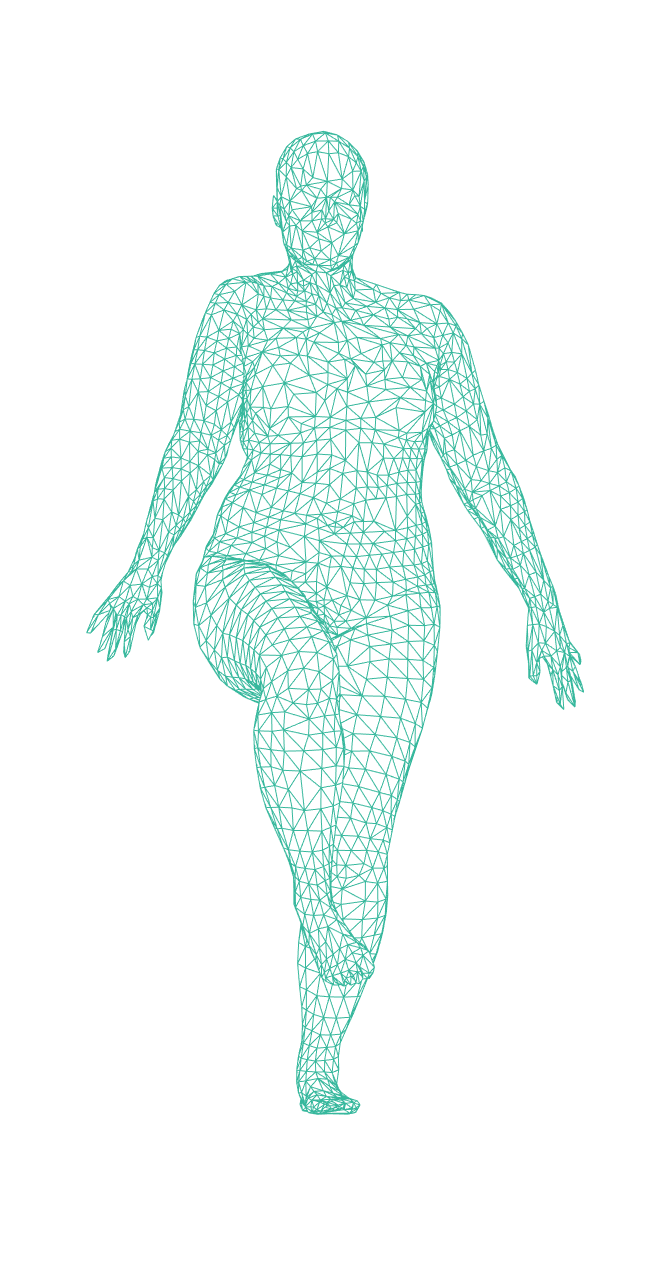}
\end{tabular}
\caption{On the left we show the receptive field at the n-1 layer before embedding corresponding to a few different vertices. On the right is a visualization of an input $3446$-vertex mesh used in our experiments.} 
\label{fig:receptive_field}
\end{figure}

\paragraph{Faces}
For the experiment using deformable faces, we used $2000$ training shapes randomly generated using the face model made available in~\cite{gerig2017morphable}. To generate missing patches (see Figure 9, top row) we remove vertices from randomly placed rectangular regions of size $0.3W$-by-$0.3H$, where $W,H$ are the width and height of the face mesh. We sample $4$ such rectangular patches for each face mesh, allowing for overlap. The hyperplane cuts shown in Figure 9, row 3, are generated by randomly orienting a hyperplane through the mesh centroid. For noisy correspondences (Figure 9, rows 5 and 7) we randomly permute a percentage of the ordered mesh vertices (recall this ordering determines the correspondence used to compute the loss during shape completion optimization). We will make all training shapes and partial evaluation shapes available for download.

\subsection{Error maps for range scan completion}
The top two rows of Figure~\ref{fig:proj_completion_appendix} reproduce the images from Figure~\ref{fig:proj_completion}. Here, we add an additional row showing an error heatmap for each of the four completion techniques for the partial input depicted in the second row. The heatmaps are shown on the ground truth complete shape as reference, and the values indicate the Euclidean error for unseen vertices. Please zoom into the figure to see the scale. 
\begin{figure*}[ht]
\centering
%\vspace{12pt}
\addtolength{\tabcolsep}{-4pt}
\begin{tabular}{cccccc}
Input & Ground truth & Poisson & NN & 3D-EPN & Ours \\[4pt]
\includegraphics[height=0.19\textwidth]{./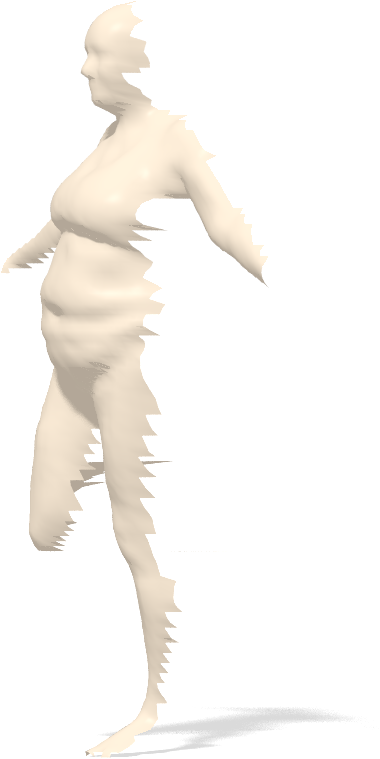} & 
\includegraphics[height=0.19\textwidth]{./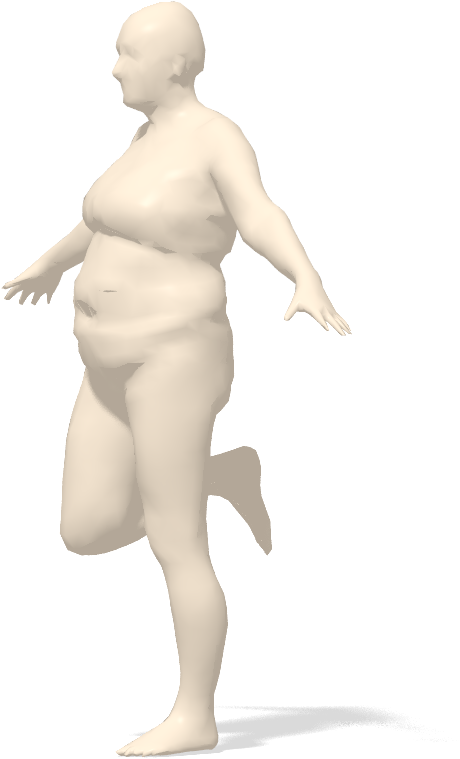} & 
\includegraphics[height=0.19\textwidth]{./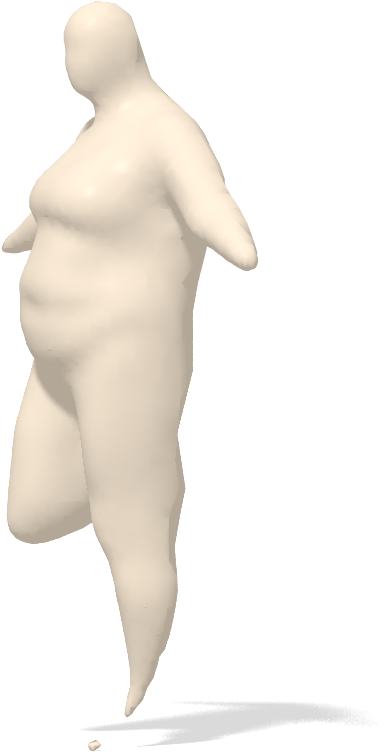} &  
\includegraphics[height=0.19\textwidth]{./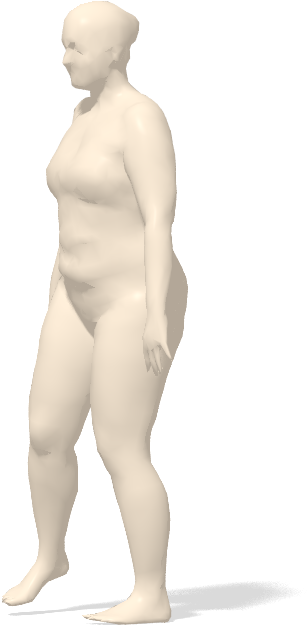} &  
\includegraphics[height=0.19\textwidth]{./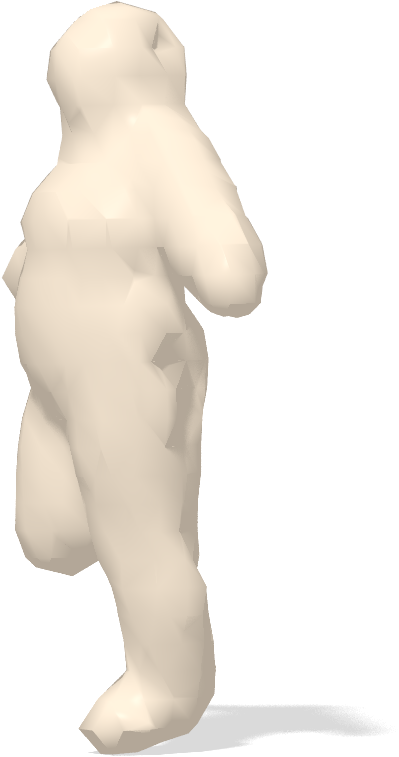} &  
\includegraphics[height=0.19\textwidth]{./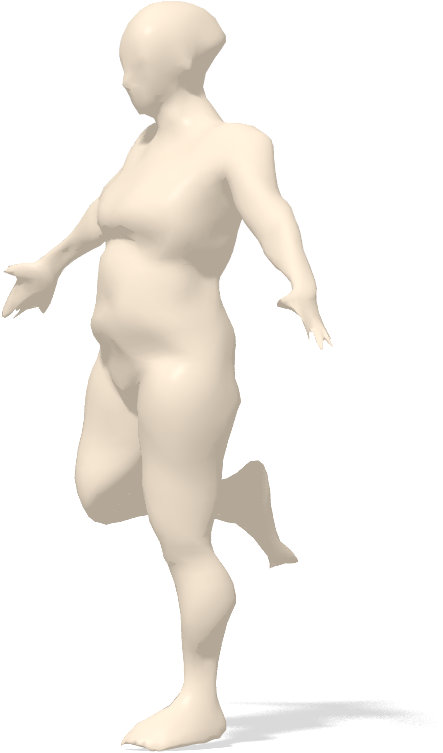} \\[4pt]
\includegraphics[height=0.19\textwidth]{./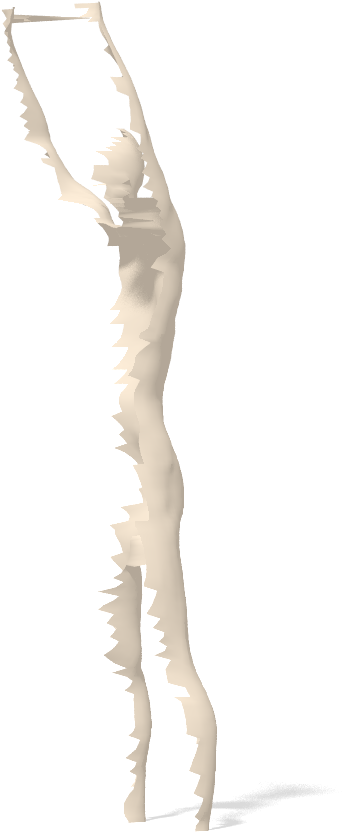} &
\includegraphics[height=0.19\textwidth]{./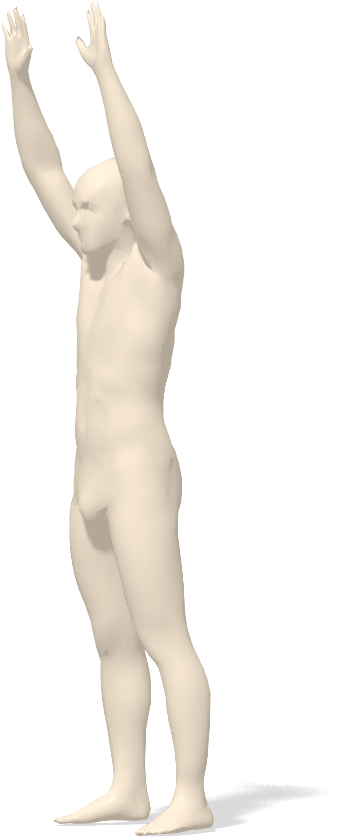} &
\includegraphics[height=0.19\textwidth]{./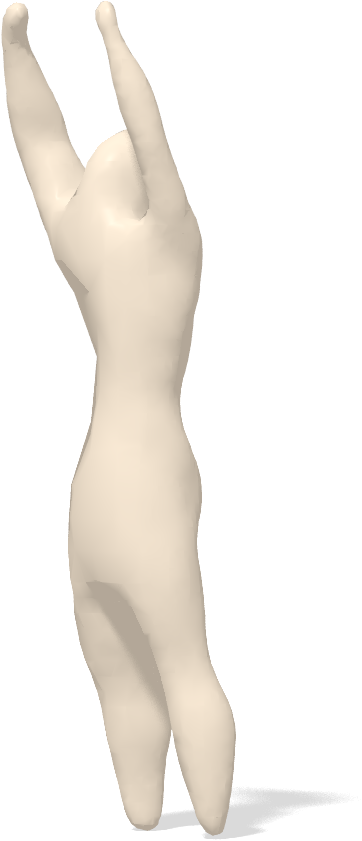} &
\includegraphics[height=0.17\textwidth]{./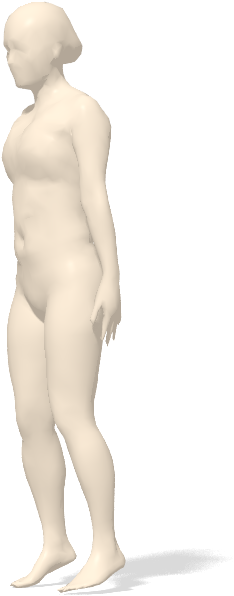} &
\includegraphics[height=0.19\textwidth]{./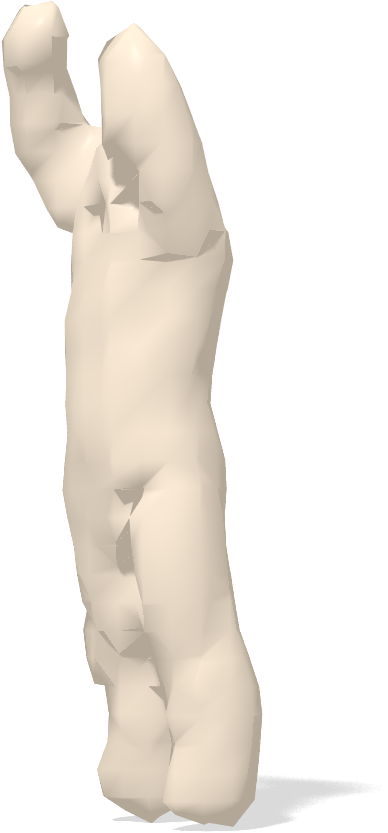} &
\includegraphics[height=0.19\textwidth]{./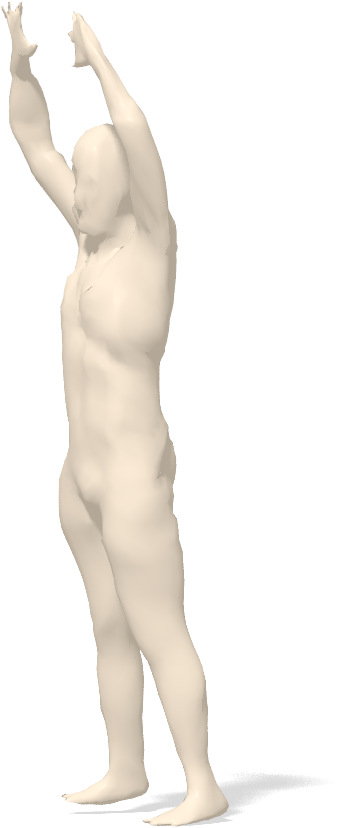} \\[4pt]
& \includegraphics[height=0.19\textwidth]{./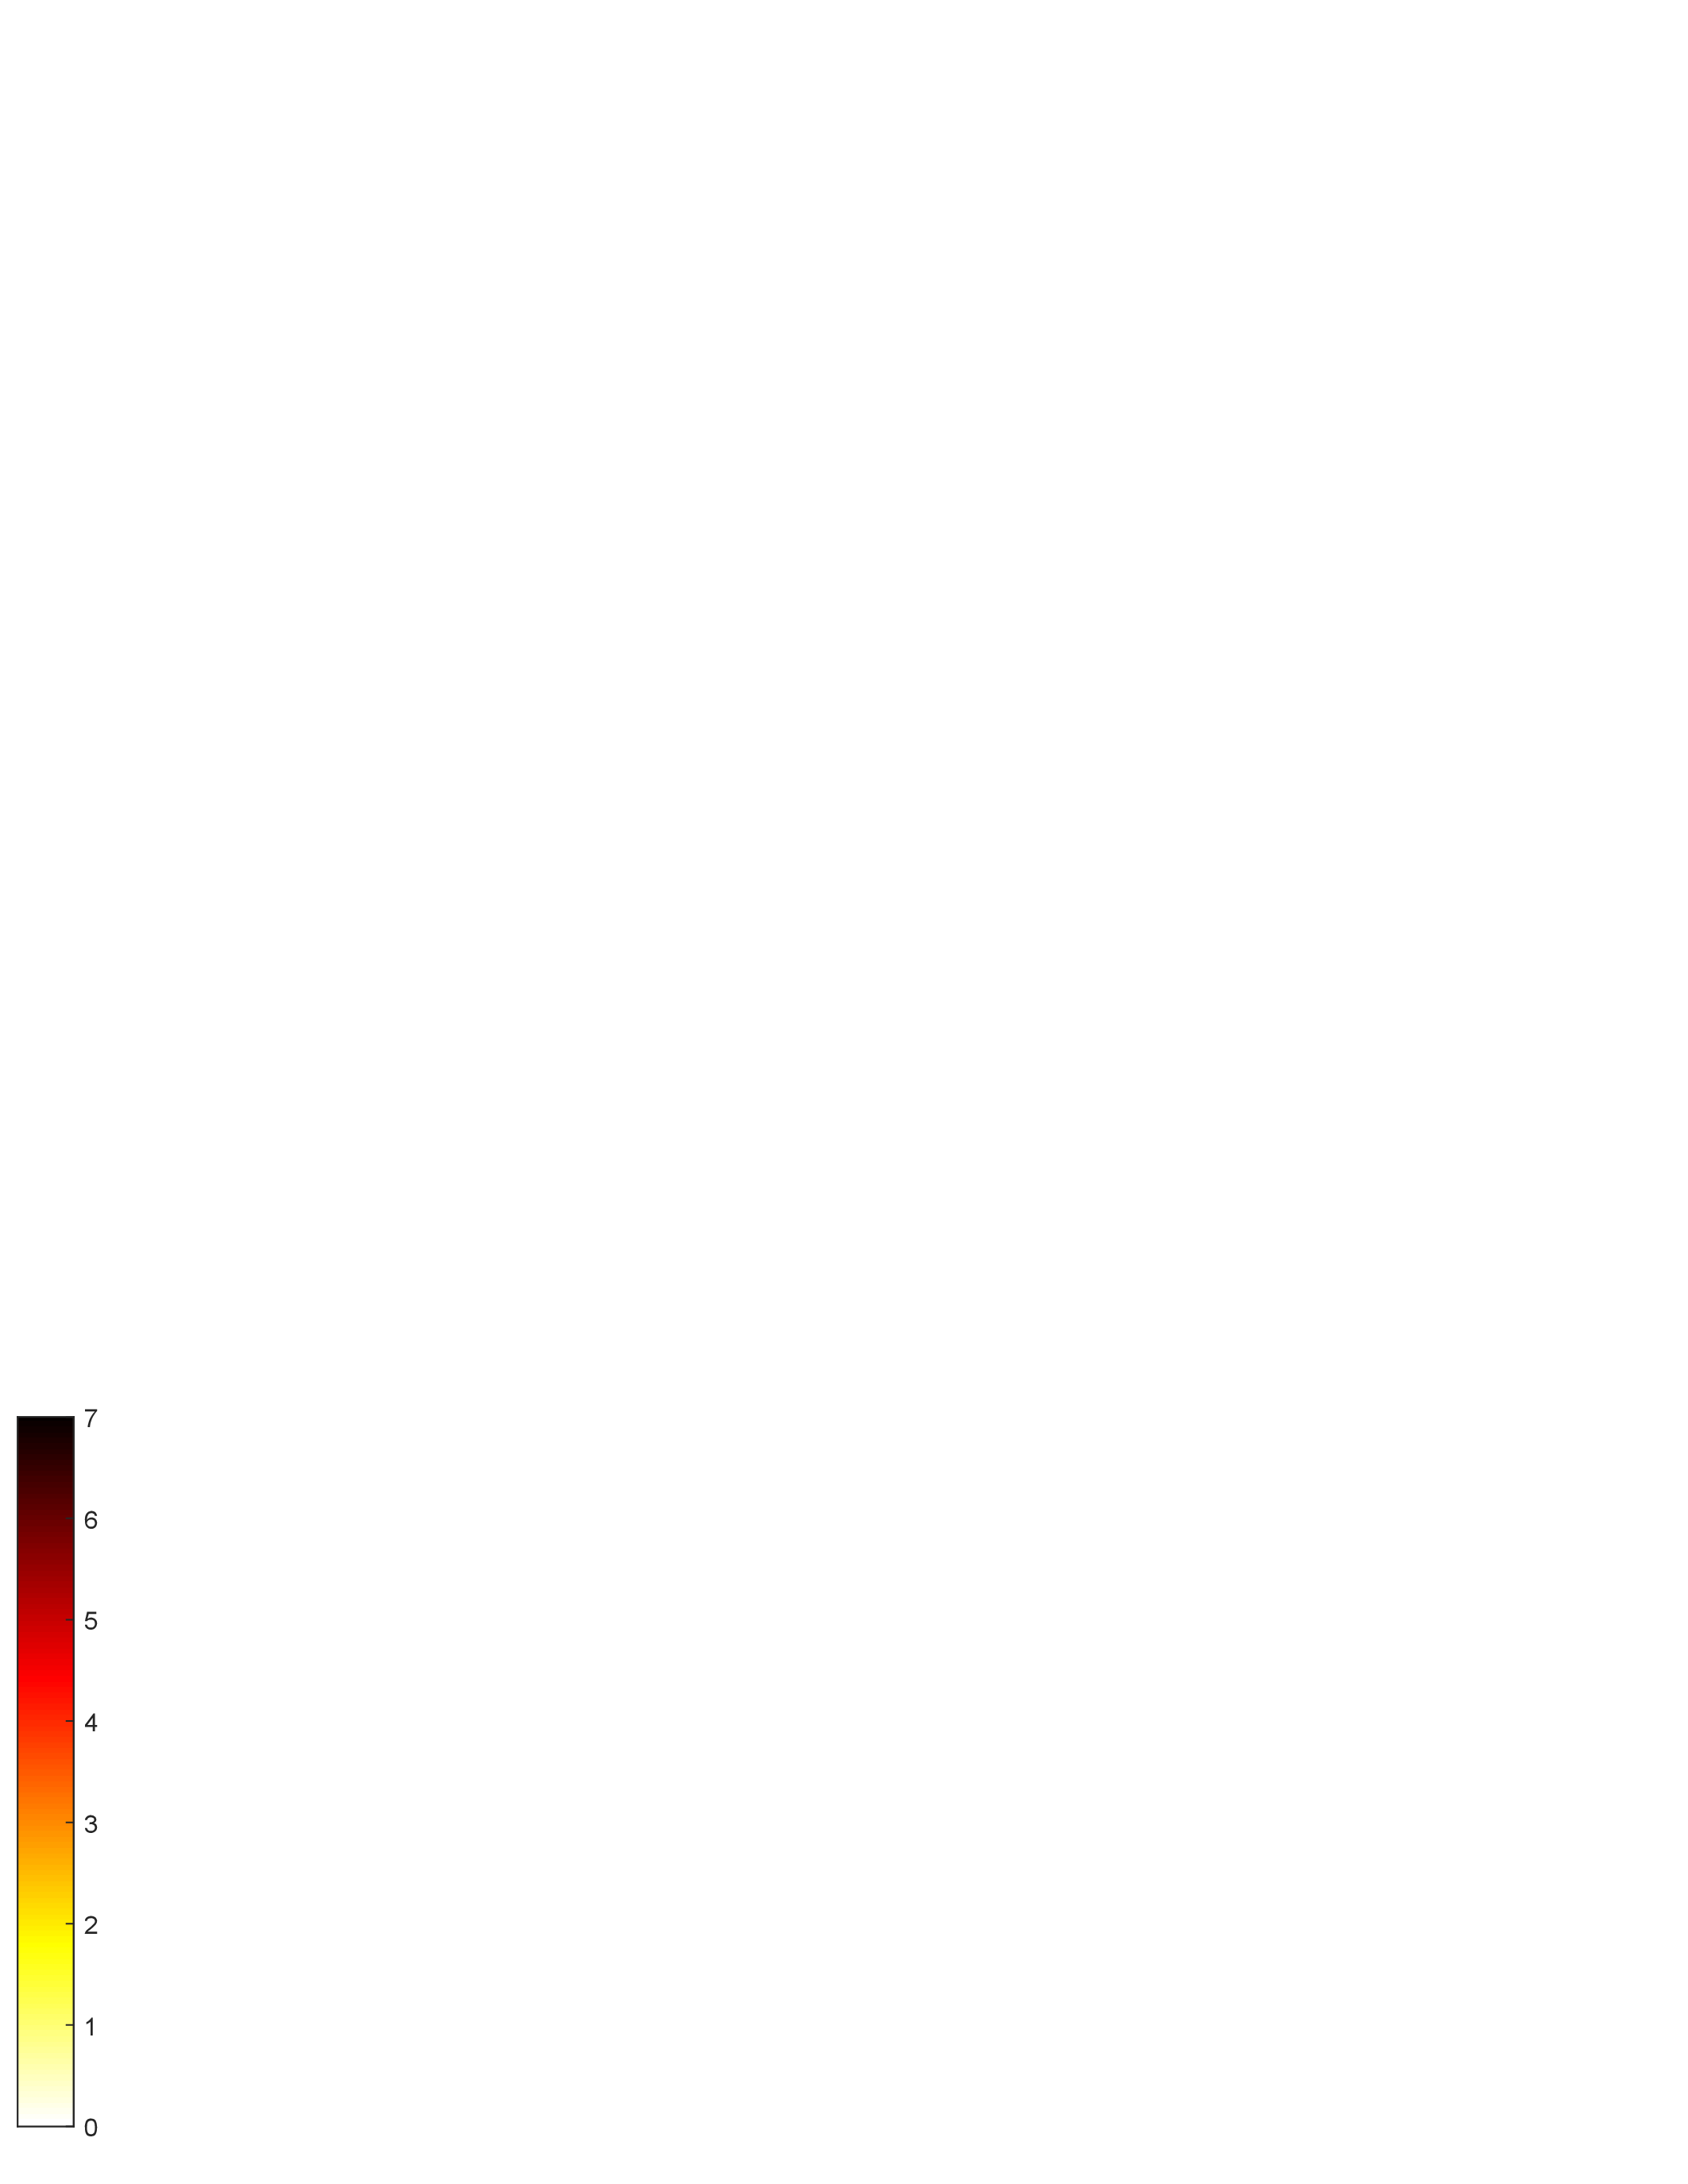} & \includegraphics[height=0.19\textwidth]{./figures/ptwise_err_poiss.png} & \includegraphics[height=0.19\textwidth]{./figures/ptwise_err_nn.png} &
\includegraphics[height=0.19\textwidth]{./figures/ptwise_err_voxnet.png} & 
\includegraphics[height=0.19\textwidth]{./figures/ptwise_err_ours.png} 
\end{tabular}
\vspace{2mm}
\caption{Comparison of different synthetic range scan completion methods. From left to right: input range scan, ground truth complete shape, Poisson reconstruction~\cite{kazhdan2013screened}, NN completion, 3D-EPN~\cite{dai2016shape}, and our method. 
%Bottom row shows pointwise errors between the ground truth and the completed shapes on the unseen parts.
} 
\label{fig:proj_completion_appendix}
\end{figure*}

\subsection{Input correspondences for real range scans}
In the main text we demonstrate a couple of completions on real data, taken from the MHAD dataset~\cite{ofli2013berkeley}. In an attempt to find dense correspondences between the point cloud extracted from the Kinect sensor and a model of a human, we have noticed that off-the-shelf descriptors such as SHOT~\cite{tombari10}, HKS~\cite{sun2009concise} and WKS~\cite{aubry2011wave}, did not transfer well between the partial point cloud and the full mesh domains. Improved descriptors can of course be learned as was proposed by~\cite{fmnet,monet} however this is outside the scope of the work presented here. Thus we chose an ah-hoc solution in which a model of some human in a similar pose was roughly aligned to the point cloud manually, providing us with initial correspondences for the completion procedure (after rough alignment the corresponding points are found via extrinsic closest points). While such correspondences will not be perfect they will be sufficient as initialization to our method since we also utilize correspondence refinement during optimization (described in the main text). Note, the reference model used for finding input correspondences is then discarded and not used during the shape completion process. In Figure~\ref{fig:real_corr} we show the 
input point cloud on the left, along with the model used as reference in the middle. Corresponding points are colored the same. On the right hand side, we show the completed shape. It might be tempting to think that if a reference model is used for generating the correspondence input it could also be used for completion. However, as observed in the main text the nearest neighbor completion performance is quite poor, and furthermore it can be clearly seen that the final completed shape differs from the reference shape in both pose (notice the bent knees and bent elbows) and body shape (notice the thicker body type which clearly fits better the input point cloud). We are using a roughly pose-aligned shape only to generate input correspondences.
\begin{figure}[th]
\centering
\begin{tabular}{ccc}
Input point cloud & Reference model & Completed \\[4pt]
\includegraphics[height=0.3\textwidth]{./figures/corr_pcl_3.png} &
\includegraphics[height=0.3\textwidth]{./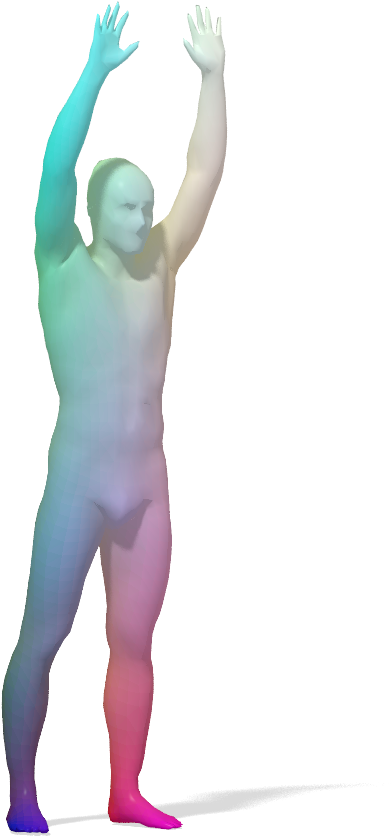} &
\includegraphics[height=0.3\textwidth]{./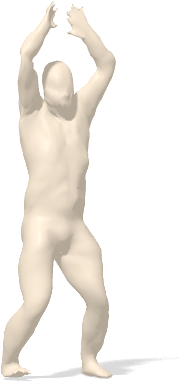}
\end{tabular}
\caption{Dense correspondence for the real data experiment were found via manual rough alignment of a reference model (middle) in a similar pose to the input point cloud (left). Corresponding points are colored the same. The completed shape is presented on the left, exhibiting different pose and body shape than the reference model.} 
\label{fig:real_corr}
\end{figure}

\subsection{Robust optimization and improved correspondences}
In Section 4.3 paragraph ``Robust optimization'', we describe a correspondence refinement technique to address noisy input correspondences during the proposed shape completion optimization. As stated, a pleasant side-effect of this refinement step is that our shape completion method can be used to obtain a de-noised (albeit sparser) correspondence set. Figure~\ref{fig:monet_refine} provides an analysis of this phenomenon as geodesic error to the true correspondences is reduced for a sparse set of vertices. To this end, we apply our shape completion algorithm using the input correspondences from MoNet \cite{monet}. Thanks to our learned shape space which acts as a prior in the optimization process, our method can handle a certain amount of outliers and noise. These can be detected by measuring the extrinsic distance between each point and the completed shape. Large distances may indicate erroneous correspondence. Such information may be used for developing powerful correspondence denoising methods but here we only show as a proof-of-concept that removing these points altogether, results in a much more accurate subset of correspondences.   

\begin{figure}[th]
\centering
\includegraphics[width=0.35\textwidth]{./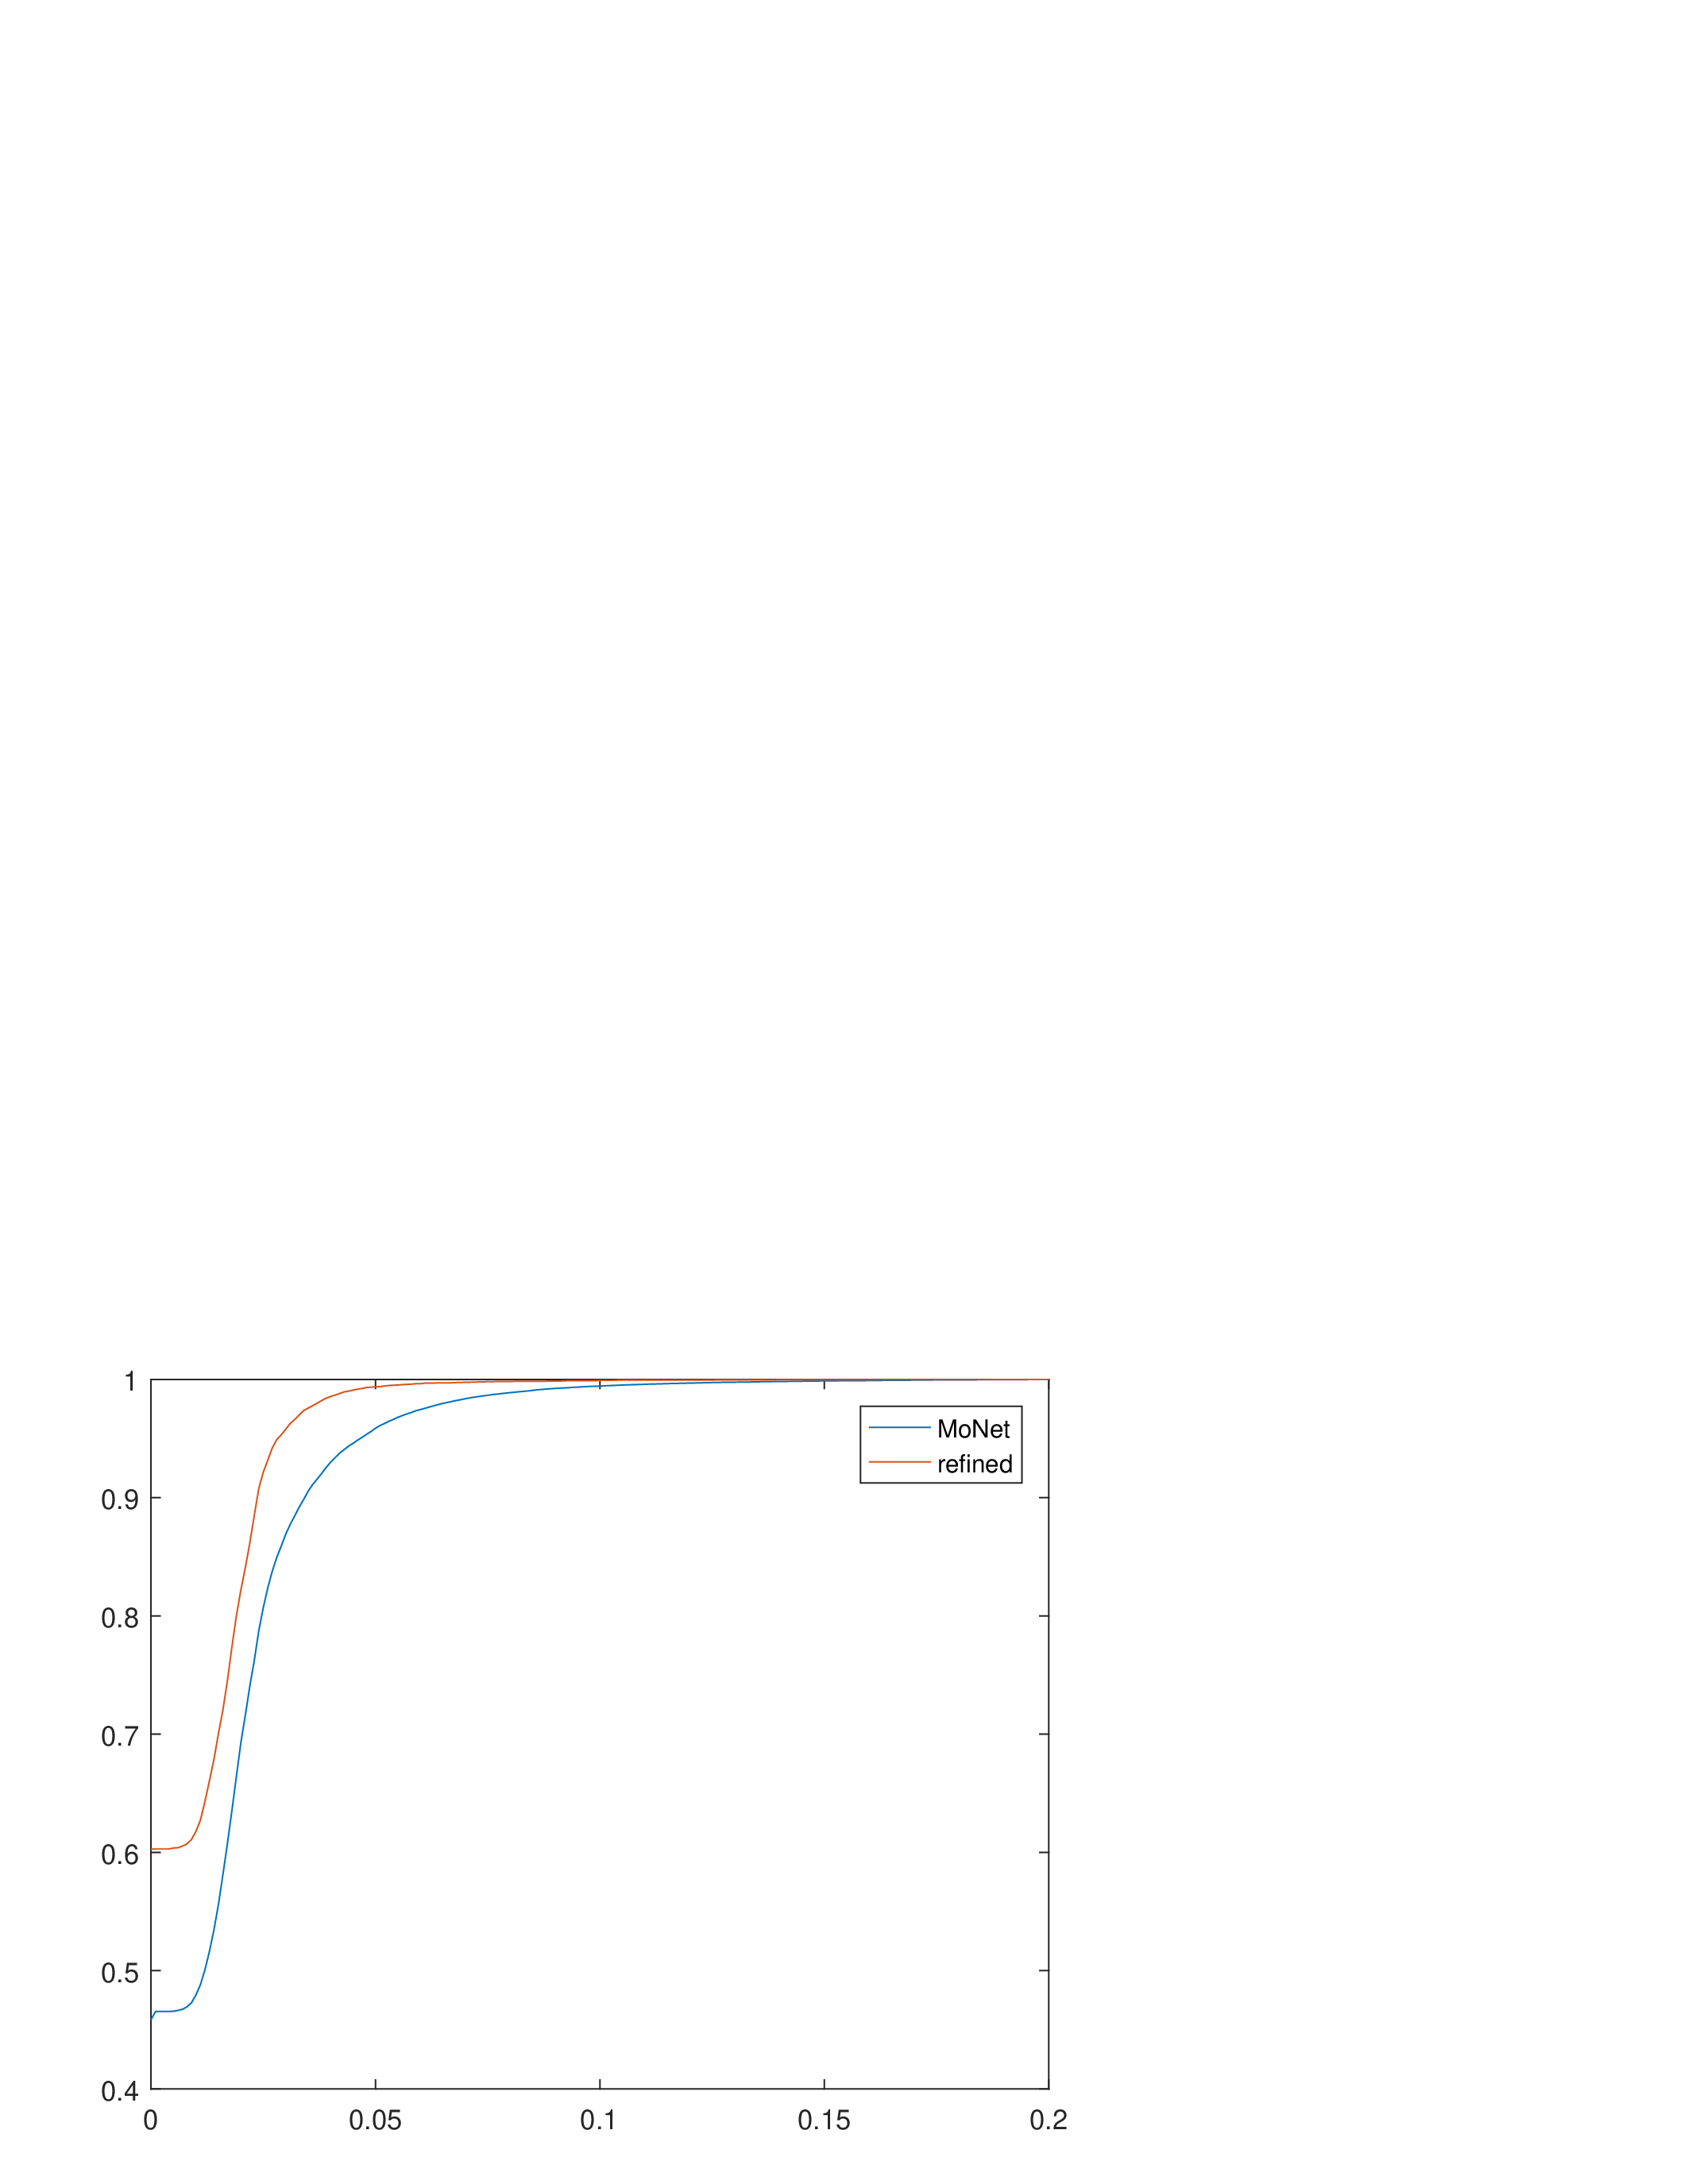}
\caption{Correspondence refinement. Keeping only correspondences of points exhibiting small Euclidean distance to the completed shape results in a distillation of the original correspondences. Quality of correspondence is plotted for each error value, as the fraction of correspondences with error smaller that that value. Errors are measured as geodesic distance from ground truth, normalized by the shape radius.} 
\label{fig:monet_refine}
\end{figure}

\subsection{Implementation details for competitors}
In the main text we report shape completion results for 3 different techniques as comparison: nearest neighbor with ground truth (referred to as NN), Poisson reconstruction~\cite{kazhdan2013screened}, and 3D-EPN~\cite{dai2016shape}.
For nearest neighbor with ground truth, we search over the entire collection of shapes seen at training. The optimal rigid transformation is computed between the partial range scan and the corresponding region of each complete training shape using ground truth correspondences. The training shape with the lowest mean Euclidean distance after alignment is chosen as the best match and completed shape. In the tables of the main text we report the mean Euclidean distance on the unseen region (like we do for all other methods). %

For Poisson reconstruction we used the MeshLab implementation of~\cite{kazhdan2013screened} with the following parameters (we manually looked for the best parameters on a small set of scans). \textit{Octree Depth} = $8$, \textit{Solver divide} = $6$, \textit{Samples per Node} = $1$, \textit{Surface offsetting} = $1.5$. %

For comparison with 3D-EPN~\cite{dai2016shape} we follow closely the details provided in the paper and the code available online. Demonstrating the performance on a single class of objects, we omitted the ``3D shape classification network'' whose output is concatenated to the encoder result to enrich it with class information. We used $32$ output features at the first layer, resulting in a latent space size of $256$. $2$ channels are provided at input: TSDF and visibility mask. Note that while having the view-angle (and hence the visibility mask) at our disposal is a valid assumption for range scan completion, it ceases to hold for general purpose completion. Nevertheless, to keep as close as possible to the original paper we allow this additional information. We also train 3D-EPN on only range-scans providing the network with a strong prior on the type of partiality. The output voxel tsdf grid size is $32^3$ as in the original work, from which we apply Matlab's isosurface function. As with all other methods error is calculated only on the unseen part of the shape. Note, the full algorithm presented in~\cite{dai2016shape} includes a post-processing refinement step (to take the network's output $32^2$ discretization up to $128^3$). We omit this data-driven nearest neighbor refinement scheme here for multiple reasons: (1) it is unclear how to best define the shape and patch matching in our setting of deformable models. The 3D-CNN for nearest neighbor shape retrieval, and the voxel/patch correspondence features, would likely need to be altered for deformable shape matching. (2) The hierarchical refinement step will be improving the resolution but also altering the completed shape, and in general a data-driven shape refinement could be applied to any shape completion technique including ours. We leave it to future work for a separate evaluation of refinement schemes for shape generation and completion. 

\subsection{Shape completion convergence}
Figure~\ref{fig:convergence} illustrates the convergence properties for the proposed shape completion optimization. Please refer to the caption for details. 
\begin{figure}[th]
\centering
\includegraphics[width=0.35\textwidth]{./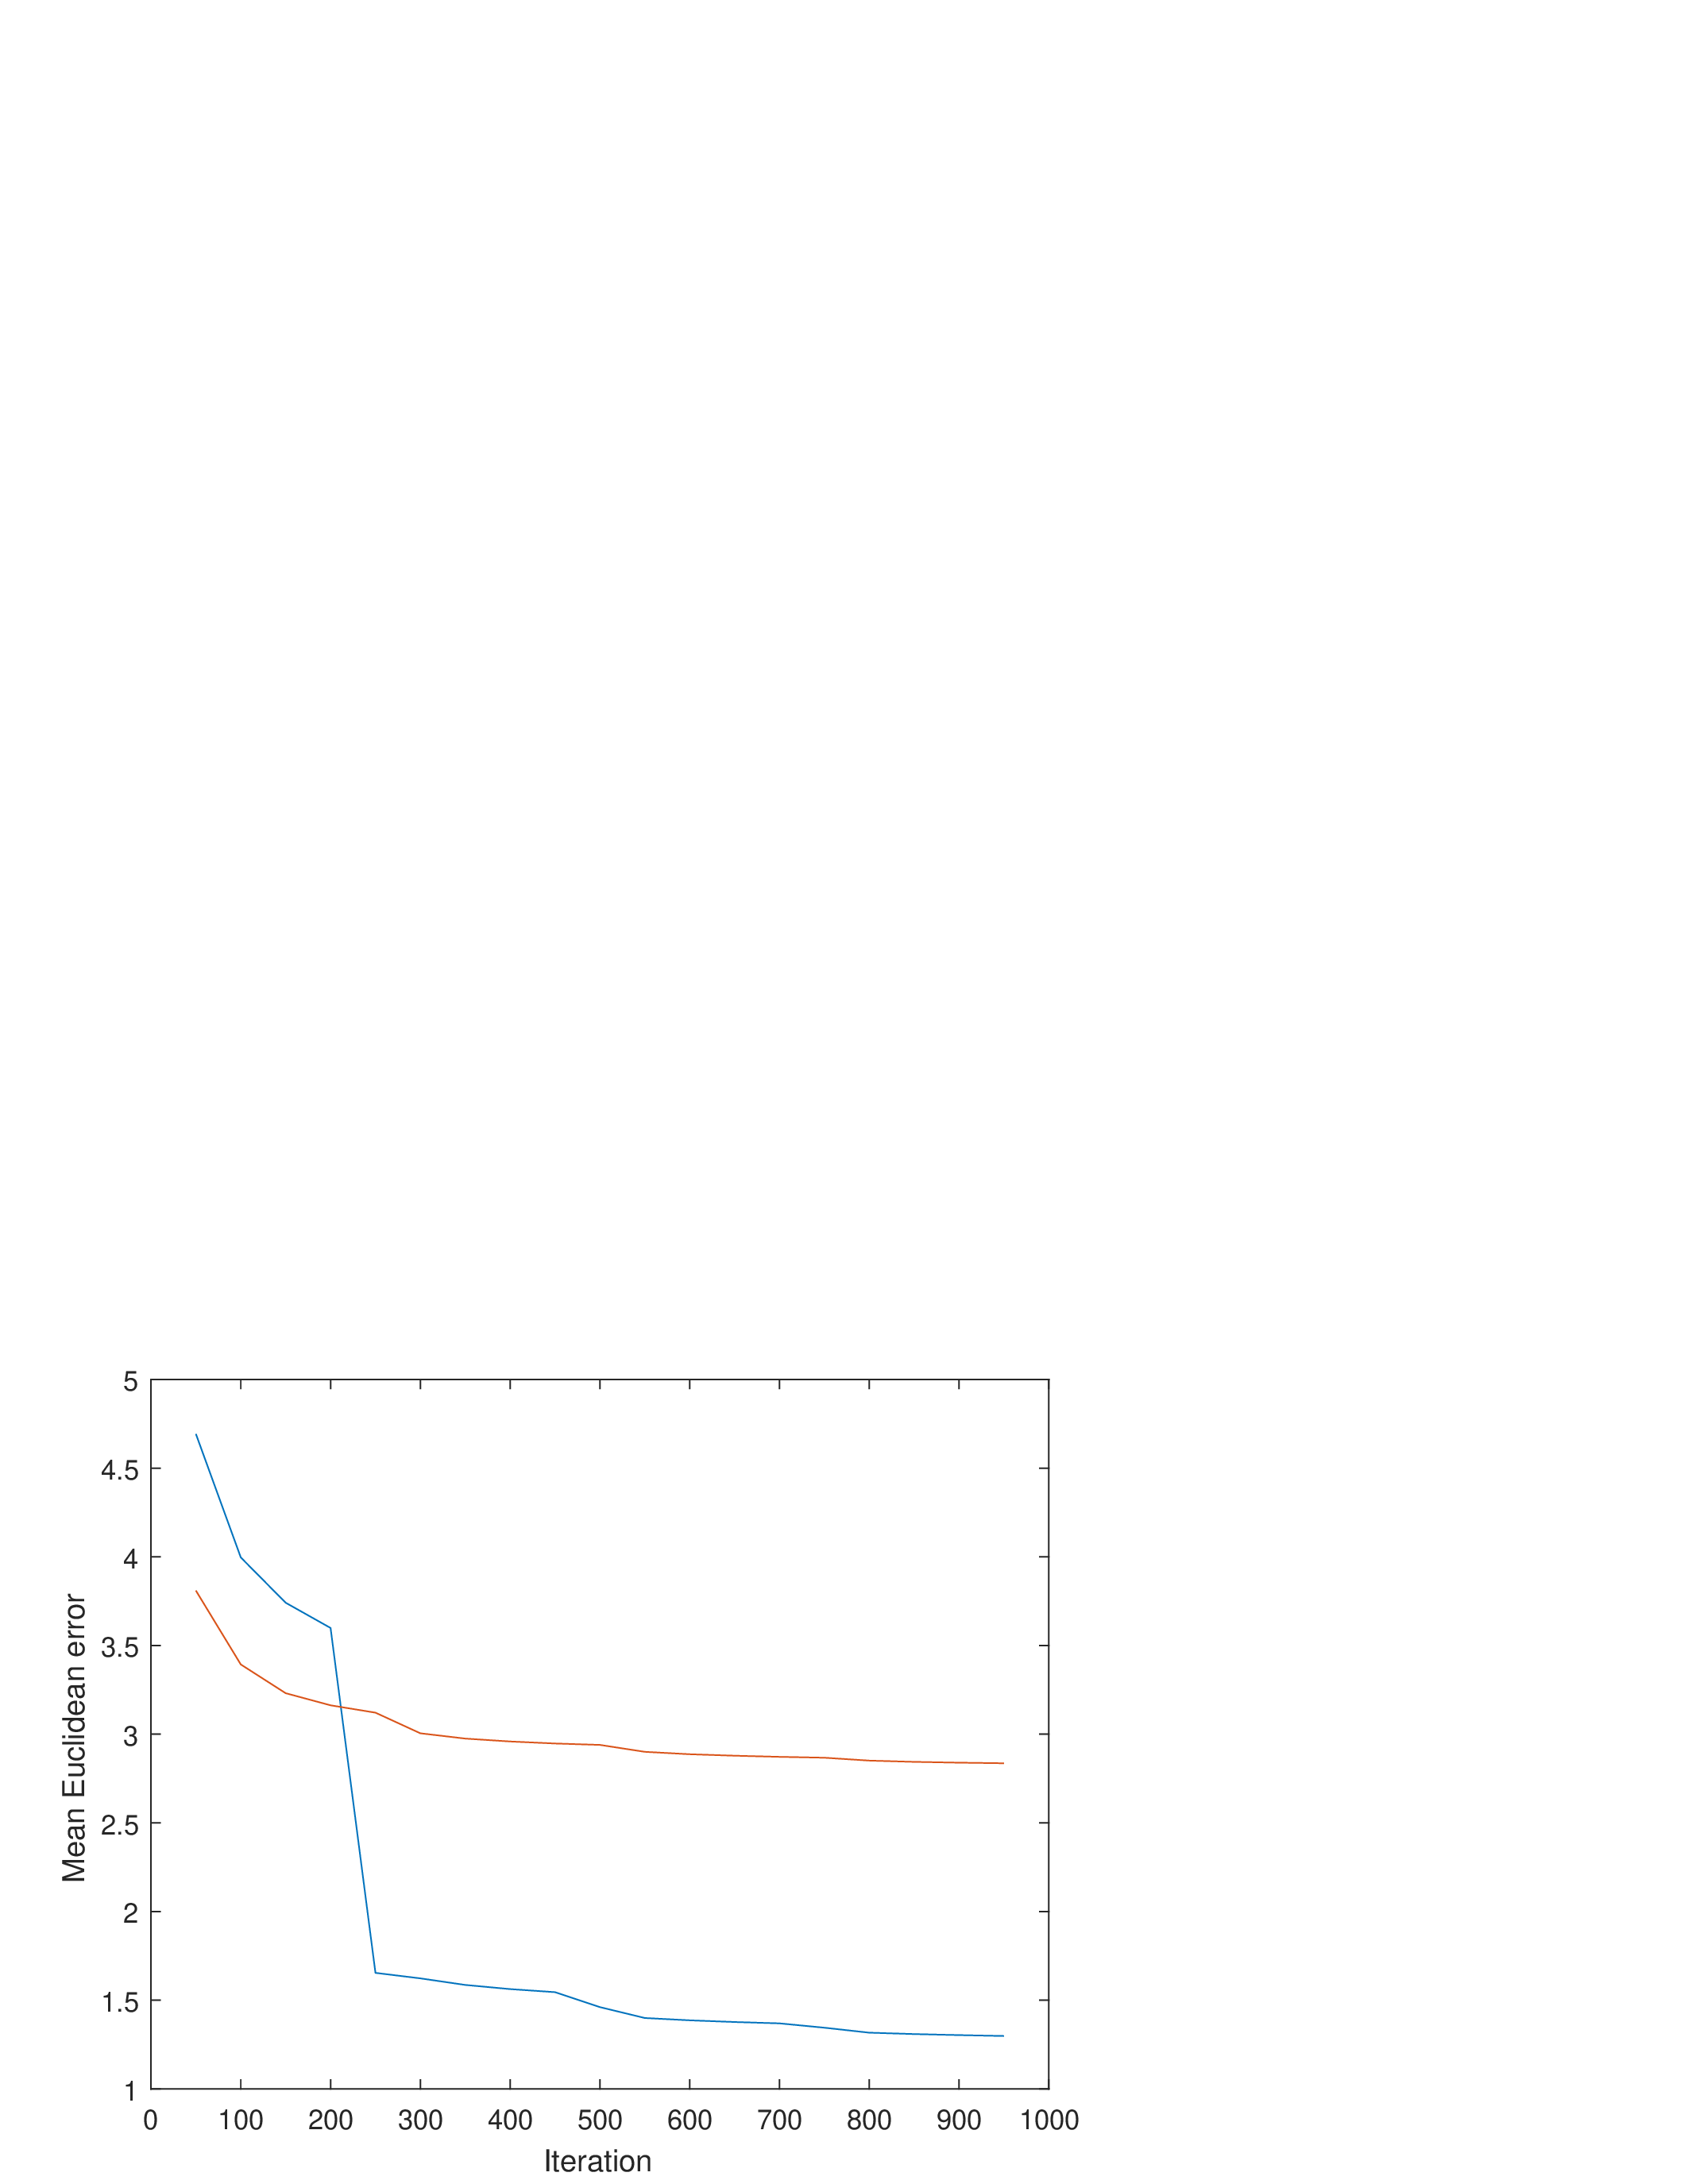}
\caption{This plot illustrates the convergence properties of the proposed shape completion method. The errors shown are averaged over all 200 test subjects (see Section 4 of the main text). The blue line shows the error between the visible partial shape and the current completed shape using the input correspondences. Note, noisy input correspondences will be reflected in this error. For this evaluation the correspondence refinement step was executed at iteration 250 for each partial shape, and this leads to the large drop in error. The red line shows the error on the unseen part which is the metric we are interested in for completion and is reported in the evaluation tables. A nice property here is the roughly monotonically decreasing error.} 
\label{fig:convergence}
\end{figure}

\subsection{Additional results for completing partial human shapes}
To provide additional insight into the proposed shape completion procedure, we visualize the completed shape at different iterations. Figure~\ref{fig:progression} displays shapes at iterations $50, 100, 150, 200$ and $950$. The vertices are colored according to the Euclidean distance from the corresponding vertex on the groundtruth. Mean Euclidean errors on the entire shape are reported as well. As noted in the figure caption, while the Euclidean error continues to decrease slightly during the later iterations, the shape and pose converge quickly from a perceptive standpoint.

In Figure~\ref{fig:recon_overlay} we show a completion example where the partial input comes not from a range scan but a manual removal of large contiguous regions of the body (in this case both arms and the entire lower body). In this figure we show the completed shape overlaid with the partial input to highlight how the proposed method produces completions that accurately match the body shape of the input in addition to generating plausible poses.

%showing a nice correspondence with the change in pose and body shape. 
\begin{figure*}[th]
\centering
\resizebox{1\columnwidth}{!}{
\addtolength{\tabcolsep}{-4pt}
\begin{tabular}{ccccccc}
\includegraphics[height=0.4\textwidth]{./progress_figures/gt_91.png} &
\includegraphics[height=0.4\textwidth]{./progress_figures/ptwise_err_per_step_1.png} &
\includegraphics[height=0.4\textwidth]{./progress_figures/ptwise_err_per_step_2.png} &
\includegraphics[height=0.4\textwidth]{./progress_figures/ptwise_err_per_step_3.png} & 
\includegraphics[height=0.4\textwidth]{./progress_figures/ptwise_err_per_step_4.png} &
\includegraphics[height=0.4\textwidth]{./progress_figures/ptwise_err_per_step_19.png} &
\includegraphics[height=0.4\textwidth]{./progress_figures/colorbar_0_6.eps} \\
\includegraphics[height=0.4\textwidth]{./progress_figures/gt_91_side_view.png} &
\includegraphics[height=0.4\textwidth]{./progress_figures/ptwise_err_per_step_1_side.png} &
\includegraphics[height=0.4\textwidth]{./progress_figures/ptwise_err_per_step_2_side.png} &
\includegraphics[height=0.4\textwidth]{./progress_figures/ptwise_err_per_step_3_side.png} & 
\includegraphics[height=0.4\textwidth]{./progress_figures/ptwise_err_per_step_4_side.png} &
\includegraphics[height=0.4\textwidth]{./progress_figures/ptwise_err_per_step_19_side.png} &
 \\
Groundtruth & Iteration $50$ & Iteration $100$ & Iteration $150$ & Iteration $200$ & Iteration $950$ & \\
& Mean err $3.09$ & Mean err $2.31$ & Mean err $2.09$ & Mean err $1.95$ & Mean err $1.59$ & 
\end{tabular}
}
\caption{This figure shows snapshots of the shape completion at different iterations throughout the optimization. The bottom row shows the same shapes as the top row but from a different viewpoint. Mean Euclidean errors on the entire shape are reported. As you can see, while the error continues to decrease slightly during the later iterations, the global shape and pose characteristics converge quite quickly.}
\label{fig:progression}
\end{figure*}

\begin{figure}[th]
\centering
\begin{tabular}{cc}
\includegraphics[height=0.4\textwidth]{./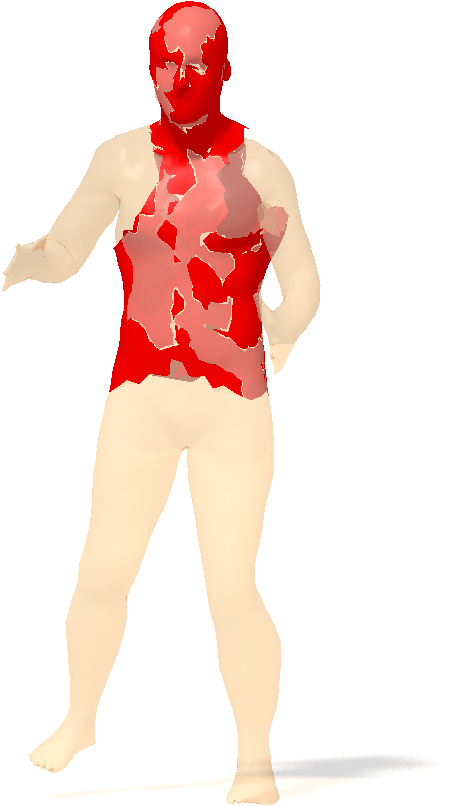} &
\includegraphics[height=0.4\textwidth]{./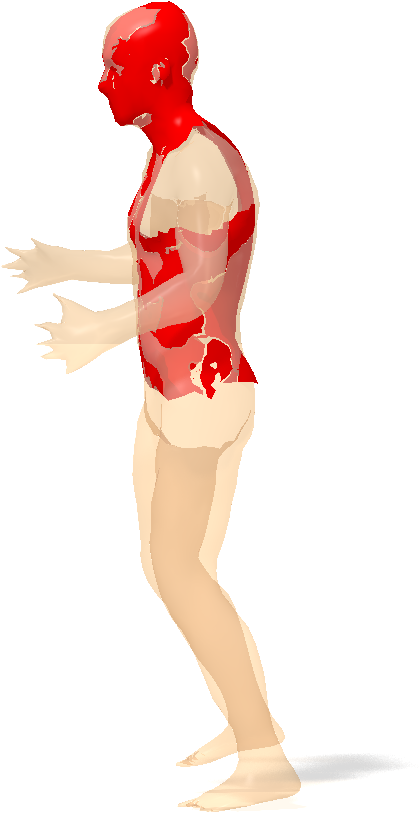}
\end{tabular}
\caption{Frontal- and side-view of the input partial shape overlaid with the completed output.} 
\label{fig:recon_overlay}
\end{figure}

\subsection{Quantitative results on faces}
Figure~\ref{fig:faces_appendix} and Table~\ref{tab:faces} show qualitative and quantitative results for shape completion on the deformable faces data (see description above). In lieu of metric scale information regarding the input meshes, error is shown as a percentage of shape radius. As expected the error increases as the correspondence noise increases.
\begin{figure}[th]
\centering
\resizebox{1\columnwidth}{!}{
\addtolength{\tabcolsep}{-4pt}
\begin{tabular}{cccccc}
\includegraphics[width=0.2\textwidth]{./face_figures/face_n05_part_00.png} &
\includegraphics[width=0.2\textwidth]{./face_figures/face_n05_part_01.png} &
\includegraphics[width=0.2\textwidth]{./face_figures/face_n05_part_02.png} &
\includegraphics[width=0.2\textwidth]{./face_figures/face_n05_part_03.png} &
\includegraphics[width=0.2\textwidth]{./face_figures/face_n05_part_04.png} \\
\includegraphics[width=0.2\textwidth]{./face_figures/face_n05_recon_00.png} &
\includegraphics[width=0.2\textwidth]{./face_figures/face_n05_recon_01.png} &
\includegraphics[width=0.2\textwidth]{./face_figures/face_n05_recon_02.png} &
\includegraphics[width=0.2\textwidth]{./face_figures/face_n05_recon_03.png} &
\includegraphics[width=0.2\textwidth]{./face_figures/face_n05_recon_04.png} &
\includegraphics[height=0.15\textwidth]{./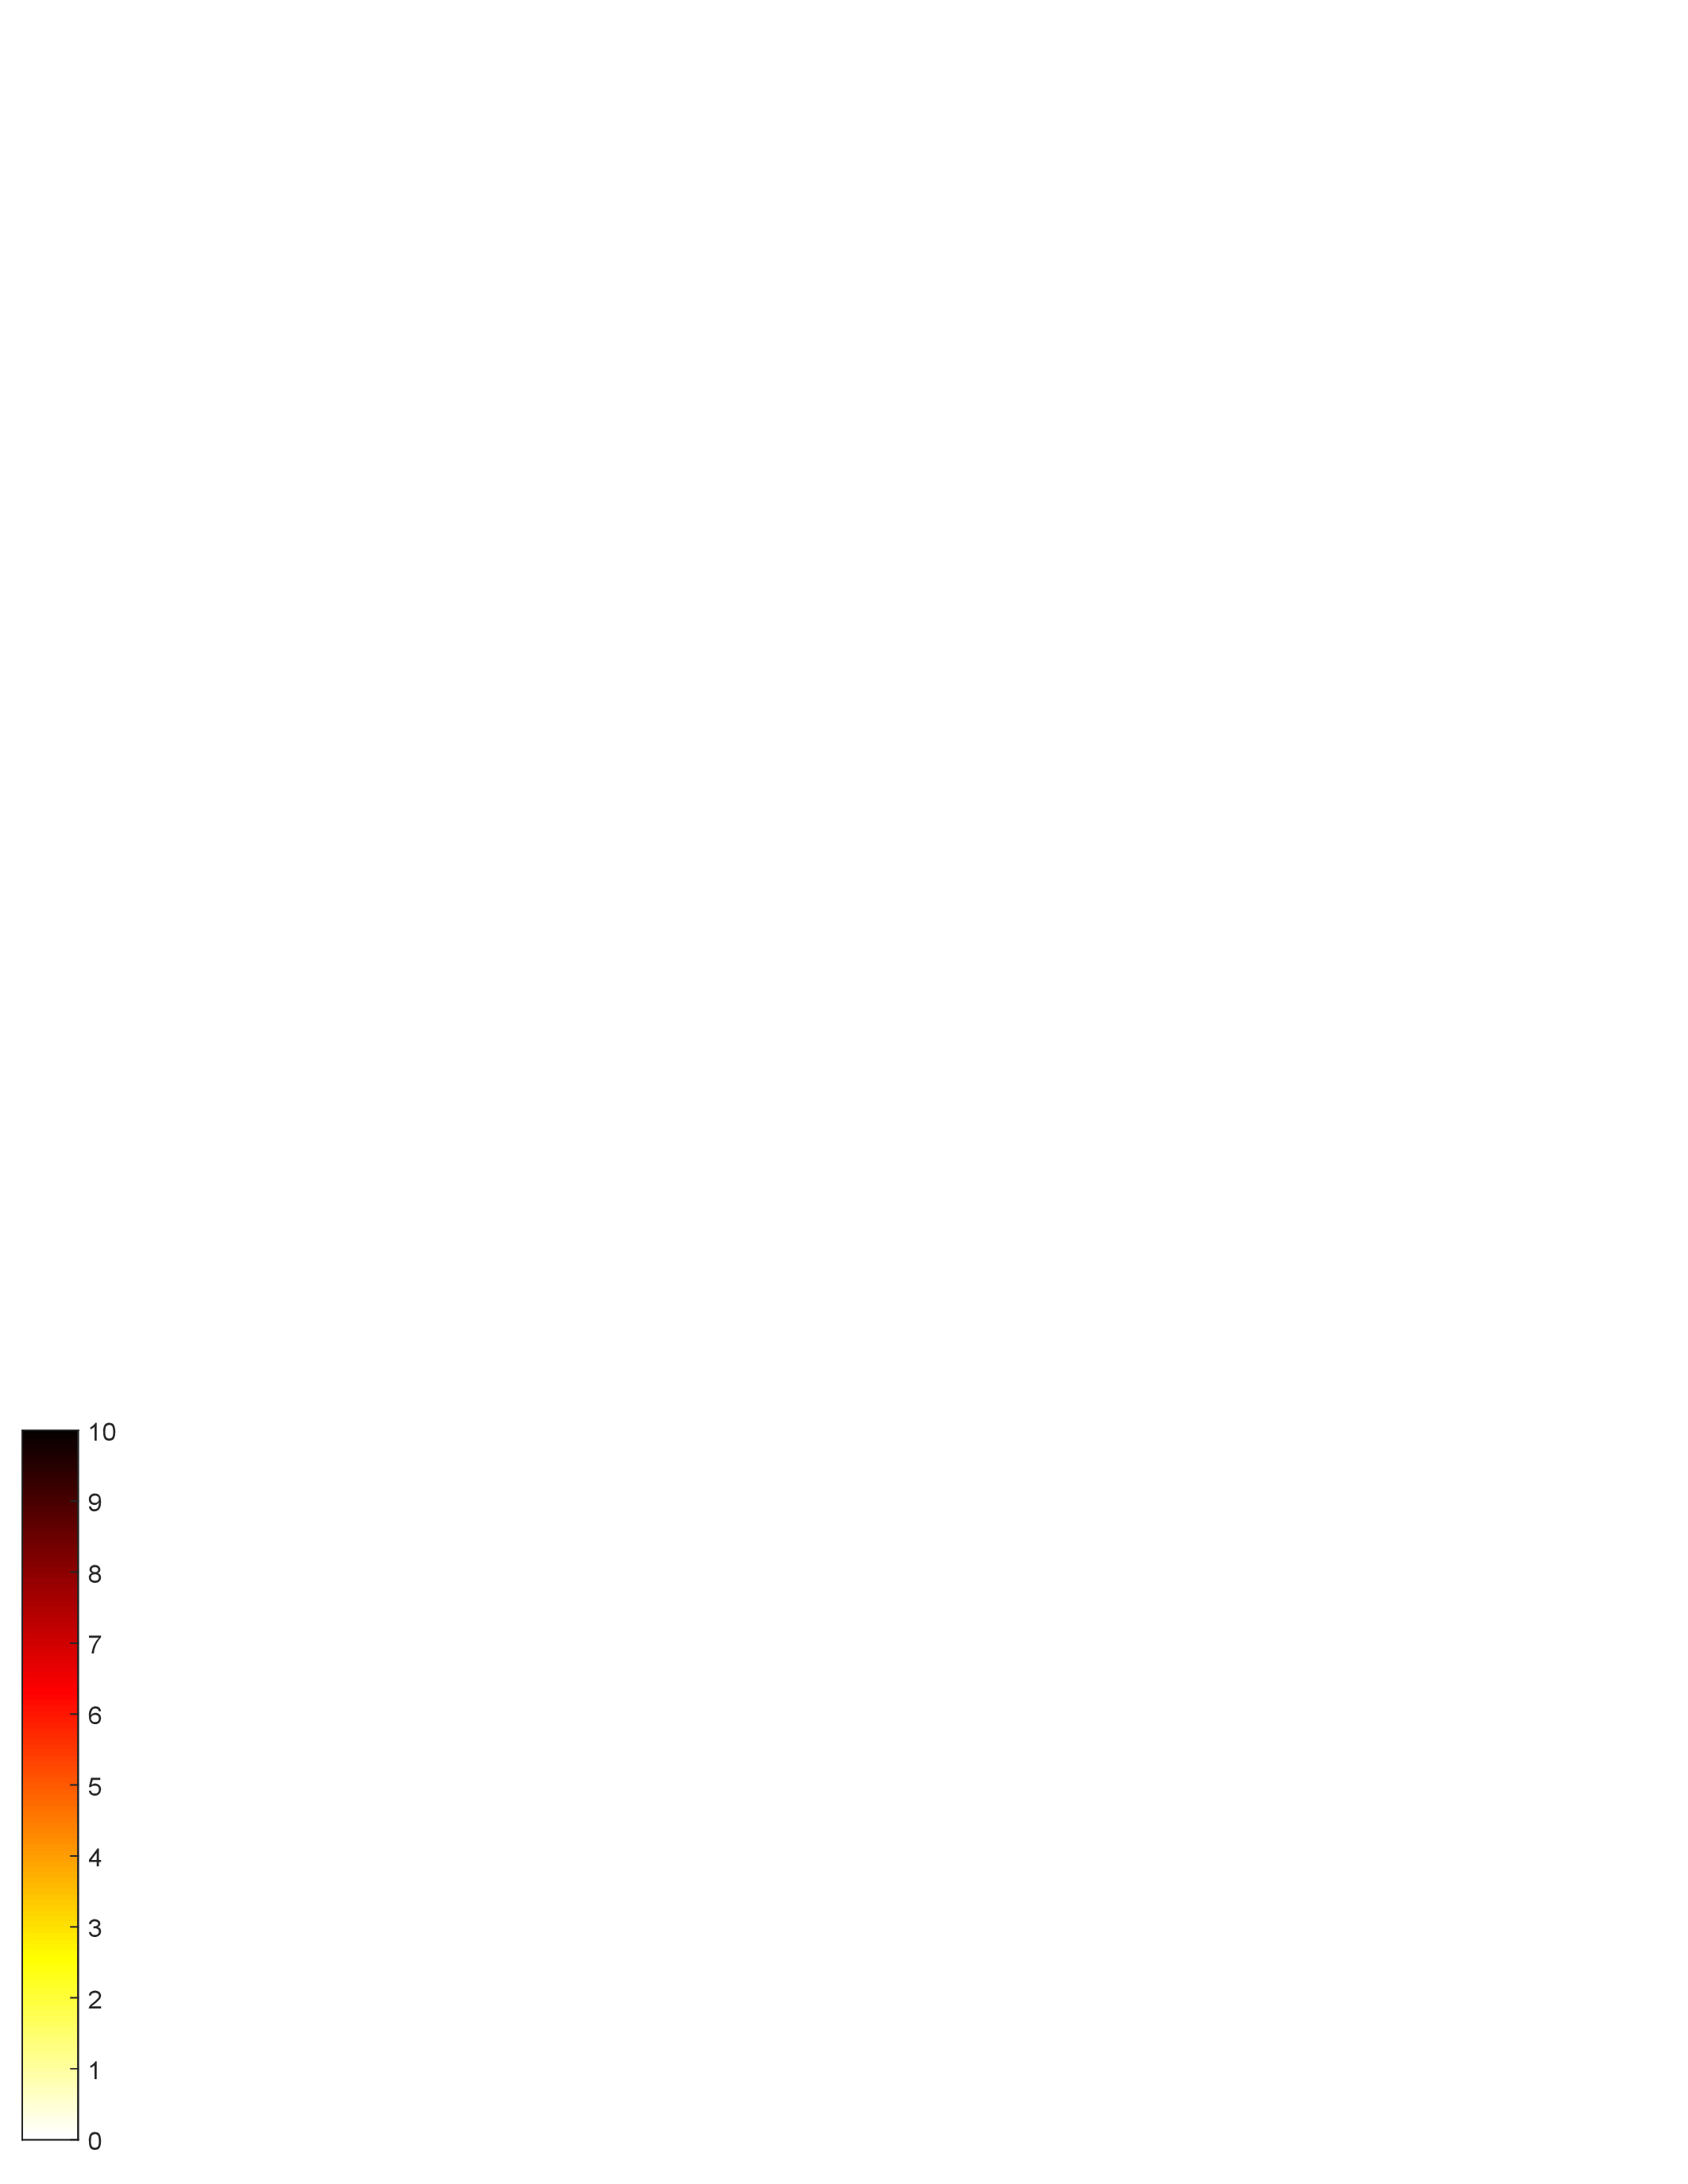} \\
\vspace{5mm}
\includegraphics[width=0.2\textwidth]{./face_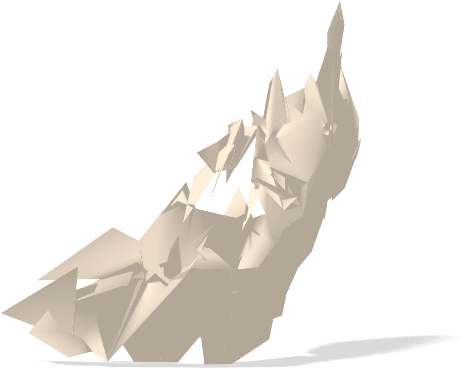} &
\includegraphics[width=0.2\textwidth]{./face_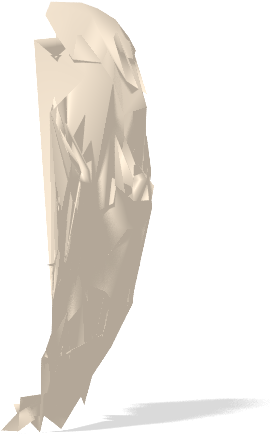} &
\includegraphics[height=0.2\textwidth]{./face_figures/face_n30_part_02.png} &
\includegraphics[height=0.2\textwidth]{./face_figures/face_n30_part_03.png} &
\includegraphics[width=0.2\textwidth]{./face_figures/face_n30_part_04.png} \\
\includegraphics[width=0.2\textwidth]{./face_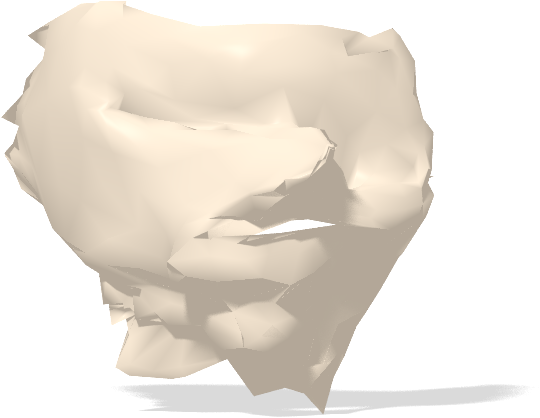} &
\includegraphics[width=0.2\textwidth]{./face_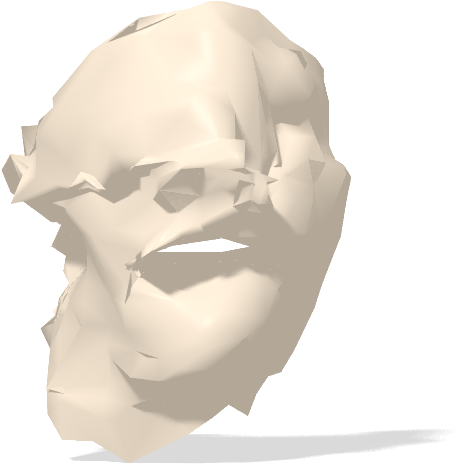} &
\includegraphics[width=0.2\textwidth]{./face_figures/face_n30_recon_02.png} &
\includegraphics[width=0.2\textwidth]{./face_figures/face_n30_recon_03.png} &
\includegraphics[width=0.2\textwidth]{./face_figures/face_n30_recon_04.png} &
\includegraphics[height=0.15\textwidth]{./face_figures/faces_colorbar.eps} \\
\end{tabular}
}
\caption{{Additional face mesh completion examples. Top rows show partial shapes with $5\%$ correspondence noise, bottom rows are with $30\%$ correspondence noise. Please zoom in to see the error heatmap scale in detail.} 
\vspace{-2mm}
} 
\label{fig:faces_appendix}
\end{figure} 
%---- faces table
\begin{table}[th]
\centering
\small
\begin{tabular}{cccc}
    \hline\hline
    Noise level & Error on seen & Err on unseen & total Err \\ \hline 
    $5\%$ & $5.76 \pm 1.8$ & $6.79 \pm 2.04$ & $6.29 \pm 1.75$\\
    $30\%$ & $8.70 \pm 2.13$ & $10.21 \pm 1.79$ & $9.42 \pm 1.37$\\   
  \end{tabular}   
  \vspace{2mm}
\caption{\small Errors on partial face mesh completion with varying levels of correspondence noise. The error is measured as percentage of the shape radius.}
\label{tab:faces}	
\end{table}
